# Supplementary material for: B4: Towards Optimal Assessment of Plausible Code Solutions with Plausible Tests
Source: arXiv:2409.08692 source file (2024-09-13)
Supplement: Supplementary file 1 [file appendix.tex]

\newpage
\clearpage

\section{Appendix}

% \section{Proofs}

In the appendix, we provide our proof for the theoretical results. We first introduce a Lemma that bounds the cumulative distribution function for normal distribution, which helps to estimate the growth rate in our subsequent analysis.
\begin{lemma}[Tails of the normal distribution]\label{thm:tail}
    For all $t>0$, we have:
    \begin{align*}
        \left(
            \frac{1}{t} - \frac{1}{t^3}
        \right)\frac{1}{\sqrt{2\pi}}e^{-\frac{t^2}{2}}\leq \Phi(-t)=1-\Phi(t)\leq \frac{1}{t}\frac{1}{\sqrt{2\pi}}e^{-\frac{t^2}{2}}.
    \end{align*}
    where $\Phi$ is the cumulative distribution function (CDF) of the standard normal distribution. This means that, when $t\rightarrow +\infty$, we have:
    \begin{align*}
        \Phi(t)\sim 1-\mathcal{O}\left(\nicefrac{c^{-t^2}}{t}\right),\quad
        \Phi(-t)\sim \mathcal{O}\left(\nicefrac{c^{-t^2}}{t}\right),
    \end{align*}
    where $c=\sqrt{e}$ is a constant.
\end{lemma}

\begin{proof}
    Proof can be found in \cite[Proposition 2.1.2]{vershynin2018high}
\end{proof}

\subsection{Proof for \cref{thm:bound_b4}}

\begin{proof}
    Let $\hat P(\theta_1), \hat P(\theta_0), \hat P(\theta_x), $ and $\hat P(\theta_y)$ denote estimated prior distributions for the four parameters, and let:
    {\footnotesize
    \begin{align*}
        I_1=\int_0^1\theta_1^{n_1} (1-\theta_1)^{|\mE_1|-n_1} P({\theta_1})\mathrm{d}\theta_1,&\; \hat I_1=\int_0^1\theta_1^{n_1} (1-\theta_1)^{|\mE_1|-n_1} \hat P({\theta_1})\mathrm{d}\theta_1,\\
        I_0=\int_0^1\theta_0^{n_0} (1-\theta_0)^{|\mE_0|-n_0} P({\theta_0})\mathrm{d}\theta_0,&\; \hat I_0=\int_0^1\theta_0^{n_0} (1-\theta_0)^{|\mE_0|-n_0} \hat P({\theta_0})\mathrm{d}\theta_0,\\
        I_x=\int_0^1\theta_x^{n_x} (1-\theta_x)^{N-n_x} P({\theta_x})\mathrm{d}\theta_x,&\; \hat I_x=\int_0^1\theta_x^{n_x} (1-\theta_x)^{N-n_x} \hat P({\theta_x})\mathrm{d}\theta_x,\\
        I_y=\int_0^1\theta_y^{n_y} (1-\theta_y)^{M-n_y} P({\theta_y})\mathrm{d}\theta_y, &\; \hat I_y=\int_0^1\theta_y^{n_y} (1-\theta_y)^{M-n_y} \hat P({\theta_y})\mathrm{d}\theta_y.
    \end{align*}
    }
    Supposing $\hat P(\mE\mid \hvx, \hvy)$ and $\hat P(\hvx, \hvy)$ denote the estimated likelihood and prior based on $\hat P(\theta_1), \hat P(\theta_0), \hat P(\theta_x), $ and $\hat P(\theta_y)$. Then we have:
    \begin{align*}
        \Delta=\left|
            \frac{
                P(\mE\mid \hvx, \hvy)P(\hvx, \hvy) - \hat P(\mE\mid \hvx, \hvy)\hat P(\hvx, \hvy)
            }{P(\mE)}
        \right|,
    \end{align*}
    therefore,
    {\small
    \begin{align*}
        P&(\mE)\cdot\Delta =|P(\mE\mid \hvx, \hvy)P(\hvx, \hvy) - \hat P(\mE\mid \hvx, \hvy)\hat P(\hvx, \hvy)|\\
        &= |I_1 I_0 I_x I_y - \hat I_1\hat I_0\hat I_x\hat I_y|\\
        &=|(I_1-\hat I_1) I_0 I_x I_y + \hat I_1 (I_0 - \hat I_0) I_x I_y + \hat I_1\hat  I_0 (I_x - \hat I_x) I_y + \hat I_1\hat  I_0 \hat I_x (I_y - \hat I_y)|\\
        &\leq |I_1-\hat I_1| I_0 I_x I_y + \hat I_1 |I_0 - \hat I_0| I_x I_y + \hat I_1\hat  I_0 |I_x - \hat I_x| I_y + \hat I_1\hat  I_0 \hat I_x |I_y - \hat I_y|\\
        &\leq I_0 I_x I_y \int_0^1\theta_1^{n_1} (1-\theta_1)^{|\mE_1|-n_1} |P({\theta_1})-\hat P({\theta_1})|\mathrm{d}\theta_1 \\
        &\quad + \hat I_1 I_x I_y \int_0^1\theta_0^{n_0} (1-\theta_0)^{|\mE_0|-n_0}  |P({\theta_0})-\hat P({\theta_0})|\mathrm{d}\theta_0 \\
        &\quad + \hat I_1\hat  I_0 I_y \int_0^1\theta_x^{n_x} (1-\theta_x)^{N-n_x} |P(\theta_x) - \hat P({\theta_x})|\mathrm{d}\theta_x \\
        &\quad + \hat I_1\hat  I_0 \hat I_x \int_0^1\theta_y^{n_y} (1-\theta_y)^{M-n_y} |\hat P({\theta_y}) - P({\theta_y})|\mathrm{d}\theta_y \\
        &\leq c_1 \int_0^1 |P({\theta_1})-\hat P({\theta_1})|\mathrm{d}\theta_1 + c_0 \int_0^1 |P({\theta_0})-\hat P({\theta_0})|\mathrm{d}\theta_0\\
        &\quad+ c_x \int_0^1 |P({\theta_x})-\hat P({\theta_x})| \mathrm{d}\theta_x + c_y \int_0^1 |P({\theta_y})-\hat P({\theta_y})| \mathrm{d}\theta_y\\
        &= 2c_1 \Delta_{\theta_1} +  2c_0 \Delta_{\theta_0}  +  2c_x \Delta_{\theta_x} +  2c_y \Delta_{\theta_y},
    \end{align*}
    }
    where $\Delta_{\theta_1}=\delta(P(\theta_1), \hat P(\theta_1))$ denotes the total variation distance of two distributions $P(\theta_1)$ and $\hat P(\theta_1)$. The last inequality uses the fact that all probabilities have upper bounds (less than 1).
\end{proof}

\subsection{Proof for \cref{thm:maxpass}}

% \begin{customthm}{1}[Error analysis of \method{MaxPass}]
%     Suppose there exist $n_y$ correct test cases and $\nny$ incorrect test cases ($n_y+\nny=M$). When both $n_y$ and $\nny$ are large enough, the probability of any incorrect code passing $Y$ ($Y\geq n_y$) test cases is:
%     \begin{align*}
%         % \label{eq:maxpass_single_error}
%         P(Y\geq n_y)\sim \Phi\left(
%             \frac{
%                 \nny\theta_0+n_y(1-\theta_1)
%             }{
%                 \sqrt{n_y \theta_1(1-\theta_1)+\nny\theta_0(1-\theta_0)}
%             }
%         \right),
%     \end{align*}
%     where $\Phi$ is the cumulative distribution function (CDF) of the standard normal distribution. 
% \end{customthm}

\begin{proof}
    For any incorrect code, let $Y_\text{c}$ denote the number of correct test cases it passes out of $n_y$, and let $Y_\text{i}$ denote the number of incorrect test cases it passes out of $\nny$. Then, the desired probability $P(Y\geq n_y)=P(Y_\text{c}+Y_\text{i}\geq n_y)$.

    It is obvious that $Y_\text{c}\sim \text{Binomial}(n_y, \theta_1)$ and $Y_\text{i}\sim \text{Binomial}(\nny, \theta_0)$, where $\text{Binomial}$ denotes binomial distribution. When both $n_y$ and $\nny$ are sufficiently large, binomial distribution can be approximated by normal distribution according to \textit{the Law of Large Numbers}. Based on the mean and the variance of the binomial distribution,
    \begin{align*}
        Y_\text{c}\sim &\mathcal{N}(n_y\theta_1, n_y\theta_1(1-\theta_1)),\\
        Y_\text{i}\sim &\mathcal{N}(\nny\theta_0, \nny\theta_0(1-\theta_0)).
    \end{align*}

    Therefore,  $Y=Y_\text{c}+Y_\text{i}$ follows normal distribution as well. Since $Y_\text{c}$ and $Y_\text{i}$ are independent, we obtain:
    \begin{align*}
        Y\sim \mathcal{N}(n_y\theta_1+\nny\theta_0, n_y\theta_1(1-\theta_1) + \nny\theta_0(1-\theta_0)), 
    \end{align*}
    and accordingly,
    \begin{align*}
        Y-n_y\sim \mathcal{N}(\nny\theta_0-n_y(1-\theta_1), n_y\theta_1(1-\theta_1) + \nny\theta_0(1-\theta_0)).
    \end{align*}
    Based on the definition of $\Phi$, we can obtain our desired results, \ie, 
    \begin{align*}
        P(Y-n_y\geq 0)&=\Phi\left(
            \frac{\E[Y-n_y]}{\sqrt{\Var [Y-n_y]}}
        \right)\\
        &=\Phi\left(
            \frac{
                \nny\theta_0-n_y(1-\theta_1)
            }{
                \sqrt{n_y \theta_1(1-\theta_1)+\nny\theta_0(1-\theta_0)}
            }
        \right)
    \end{align*}
    
\end{proof}

\subsection{Proof for \cref{thm:maxpass_ny}}

% \begin{customcorollary}{{4.1}}
%     If $\theta_1<1$, then $P(Y\geq n_y)$ can exponentially converge to $0$ when $n_y\rightarrow\infty$.
% \end{customcorollary}
\begin{proof}
    Based on \cref{thm:maxpass}, denoting $P(Y\geq n_y)\sim \Phi(t)$ where $t=\mathcal{O}(\sqrt{n_y})$. If $\theta_1<1$, with the increase of $n_y$ we have $t<0$. According to \cref{thm:tail}:
    \begin{align*}
        P(Y\geq n_y)\sim \mathcal{O}\left(
            \nicefrac{
                c^{-\mathcal{O}(\sqrt{n_y})^2}
            }{
                \mathcal{O}(\sqrt{n_y})
            }
        \right)
        =\mathcal{O}\left(
            \nicefrac{
                c_1^{-n_y}
            }{
                \sqrt{n_y}
            }
        \right),
    \end{align*}
    where $c_1>1$ is some constant and $n_y\rightarrow\infty$.

    Suppose there are $\nnx$ incorrect codes. Then as $n_y\rightarrow\infty$, the accuracy of \method{MaxPass} is:
    \begin{align*}
        P(\text{\method{MaxPass} is correct})&=(P(Y<n_y))^{\nnx}\\
        &=\left\{
            1-P(Y\geq n_y)
        \right\}^{\nnx}\\
        &\sim 1-\nnx \mathcal{O}\left(
            \nicefrac{
                c_1^{-n_y}
            }{
                \sqrt{n_y}
            }
        \right)\\
        &=1-\mathcal{O}\left(
            \nicefrac{
                c_1^{-n_y}
            }{
                \sqrt{n_y}
            }
        \right),
    \end{align*}
    where we use the fact that $(1-x)^n\sim 1-nx$ when $x\rightarrow 0$.
\end{proof}

% \begin{customcorollary}{{4.2}}
%     If there are $\nnx$ incorrect codes, the accuracy of \method{MaxPass} (\ie, the probability of all incorrect codes passing less than $n_y$ test cases) can exponentially converge to $0$ with the growth of $\nnx$.
% \end{customcorollary}

\subsection{Proof for \cref{thm:maxpass_nx}}

\begin{proof}
    Based on the above proof for \cref{thm:maxpass_ny}, we have:
    \begin{align*}
        P(\text{\method{MaxPass} is correct})=\left\{
            1-P(Y\geq n_y)
        \right\}^{\nnx},
    \end{align*}
    which exponentially converges to 0 with the growth of $\nnx$.
\end{proof}

\subsection{Proof for \cref{thm:codet}}

% \begin{customthm}{2}[Error analysis of \method{CodeT}]
%     Suppose the correctness of codes and test cases are $\vx$ and $\vy$. Let $n_x=\sum \vx$ and $n_y=\sum \vy$ denote the number of correct codes and test cases, respectively. For any \textbf{incorrect} consensus set that corresponds to a prediction $\hvx$ and $\hvy$, similarly let $n_{\hat x}=\sum \hvx$ and $n_{\hat y}=\sum \hvy$. If $N$ is large, the probability of this consensus set being scored higher than the correct one by \method{CodeT} (\ie, $n_{\hat x} n_{\hat y} > n_x n_y$) follows:
%     {\small
%     \begin{align*}
%         % \nonumber
%         P(n_{\hat x}  n_{\hat y} > n_x n_y)
%         \sim \Phi\left(
%             \frac{
%                 \sqrt{N} (\theta' n_{\hat y} - \theta_xn_y)
%             }{
%                 \sqrt{n_{\hat y}^2 \theta'(1-\theta')+n_y^2 \theta_x(1-\theta_x)-2n_{\hat y}n_y \theta' \theta_x}
%             }
%         \right),
%     \end{align*}
%     }
%     where $\theta'$ is a constant, defined as:
%     \begin{align*}
%         \theta' = (1-\theta_x) \theta_1^{\hvy^\top \vy} (1-\theta_1)^{(1-\hvy)^\top\vy}{\theta_0}^{\hvy^\top (1-\vy)}(1-\theta_0)^{(1-\hvy)^\top (1-\vy)}.
%     \end{align*}
% \end{customthm}

\begin{proof}
    For any coming code solution, three cases are possible: 
    \begin{itemize}[leftmargin=*]
        \item (A) It is classified into the correct consensus set, with a probability of $\theta_x$;
        \item (B) It is classified into the incorrect consensus set mentioned in \cref{thm:codet}, with a probability of $\theta'$ (We defer the detailed computation of $\theta'$ to the end of the proof);
        \item (C) Other cases, with a probability of $1-\theta_x-\theta'$.
    \end{itemize}
    Since $N$ solutions are coming independently, the numbers of code solutions in the three cases follow a multinomial distribution. Based on the definitions of $n_x$ and $n_{\hat x}$, they are just the numbers of code solutions that are classified into case (A) and case (B), respectively. Suppose the number of code solutions in case (C) is $n_c$, then:
    \begin{align*}
        n_x, n_{\hat x}, n_c\sim \text{Mult}(N, \theta_x, \theta', 1-\theta_x-\theta').
    \end{align*}
    
    When $N$ is sufficiently large, $n_x$ and $n_{\hat x}$ follow correlated normal distributions according to \textit{the Law of Large Numbers}. Based on the mean, variance, and the correlation of multinomial distribution:
    \begin{align*}
        \E[n_x]=N\theta_x,\quad& \Var[n_x]=N\theta_x(1-\theta_x),\\
        \E[n_{\hat x}]=N\theta',\quad& \Var[n_{\hat x}]=N\theta'(1-\theta'),
    \end{align*}
    and
    \begin{align*}
        \Cov[n_x, n_{\hat x}]=-N\theta_x\theta'.
    \end{align*}
    Therefore, $n_{\hat x}  n_{\hat y} - n_x n_y$ is also follow normal distribution $\mathcal{N}(\mu, \sigma^2)$, where
    \begin{align*}
        \mu &= \E[n_{\hat x}  n_{\hat y}] - \E[n_x n_y] \\
        &= n_{\hat y}\E[n_{\hat x}] - n_y\E[n_x]\\
        &=N(\theta' n_{\hat y} - \theta_xn_y),\\
        \sigma^2&= \Var [n_{\hat x}  n_{\hat y} - n_x n_y]\\
        &= \Var [n_{\hat x}  n_{\hat y}] + \Var [n_x n_y] + 2\Cov[n_{\hat x}  n_{\hat y}, n_x n_y]\\
        &= n_{\hat y} ^2 \Var [n_{\hat x} ] + n_y^2 \Var [n_x] + 2n_{\hat y}n_y\Cov[n_{\hat x}  , n_x]\\
        &=N\left[
            n_{\hat y}^2 \theta'(1-\theta')+n_y^2 \theta_x(1-\theta_x)-2n_{\hat y}n_y \theta' \theta_x
        \right].
    \end{align*}
    Based on the definition of $\Phi$, we can obtain the desired probability $P(n_{\hat x}  n_{\hat y} - n_x n_y>0)$, \ie, 
    \begin{align*}
        P(n_{\hat x}  &n_{\hat y} - n_x n_y>0)=\Phi\left(
            \frac{\mu}{\sigma}
        \right)\\
        =&\Phi\left(
            \frac{
                N(\theta' n_{\hat y} - \theta_xn_y)
            }{
                \sqrt{N\left[
                    n_{\hat y}^2 \theta'(1-\theta')+n_y^2 \theta_x(1-\theta_x)-2n_{\hat y}n_y \theta' \theta_x
                \right]}
            }
        \right)\\
        =&\Phi\left(
            \frac{
                \sqrt{N} (\theta' n_{\hat y} - \theta_xn_y)
            }{
                \sqrt{n_{\hat y}^2 \theta'(1-\theta')+n_y^2 \theta_x(1-\theta_x)-2n_{\hat y}n_y \theta' \theta_x}
            }
        \right).
    \end{align*}

    Now, we describe how to compute $\theta'$, \ie, the probability of case (B). For case (B), the code must be incorrect (with a probability of $1-\theta_x$) and pass exactly $\hvy$.
    % The probability $\theta'$ can be expressed in:
    % \begin{align*}
    %     \theta'=(1-&\theta_x)\cdot P(\text{pass correct tests})\cdot P(\text{not pass correct tests})\\
    %     &\cdot P(\text{pass incorrect tests})\cdot P(\text{not pass incorrect tests}).
    % \end{align*}
    Specifically, it should \textit{pass} test cases indicated by $\hvy$ and should \textit{not pass} test cases indicated by $1-\hvy$. Let four index sets be defined as:
    \begin{align*}
        &S_1=\{i \in [M] \mid y_i=1,\hy_i=1\},S_2 = \{i \in [M] \mid y_i=0, \hy_i=1\},\\
        &S_3=\{i \in [M] \mid y_i=1,\hy_i=0\},S_4 = \{i \in [M] \mid y_i=0, \hy_i=0\}.
    \end{align*}
    For the passed test cases, there are $|S_1|$ correct test cases and $|S_2|$ incorrect test cases. 
    Then, the probability could be written by
    \begin{align*}
         &P(\text{pass correct tests})=\prod_{i \in S_1}P( y_i=\hy_i=1)=\theta_1^{|S_1|}=\theta_1^{\hvy^\top \vy},\\
         &P(\text{pass incorrect tests})=\prod_{i \in S_2}P( y_i=0,\hy_i=1)=\theta_0^{|S_2|}=\theta_0^{\hvy^\top (1 - \vy)}.
    \end{align*}
    For the not passed test cases, there are $|S_3|$ correct test cases and $|S_4|$ incorrect test cases, \ie, 
    \begin{align*}
          P(\text{not pass correct tests})&=\prod_{i \in S_3}P( y_i=1,\hy_i=0)\\
          &=(1-\theta_1)^{|S_3|}=(1-\theta_1)^{(1-\hvy)^\top \vy},\\
         P(\text{not pass incorrect tests})&=\prod_{i \in S_4}P( y_i=0,\hy_i=0)\\
         &=(1-\theta_0)^{|S_4|}=(1-\theta_0)^{(1-\hvy)^\top (1-\vy)}.
    \end{align*}
    Combining the above equations, we obtain:
    \begin{align*}
        \theta' &= (1-\theta_x)\cdot P(\text{pass correct tests})\cdot P(\text{not pass correct tests})\\
        &\quad\quad\cdot P(\text{pass incorrect tests})\cdot P(\text{not pass incorrect tests})\\
        &=(1-\theta_x) \theta_1^{\hvy^\top \vy} (1-\theta_1)^{(1-\hvy)^\top\vy}{\theta_0}^{\hvy^\top (1-\vy)}(1-\theta_0)^{(1-\hvy)^\top (1-\vy)}.
    \end{align*}
     
\end{proof}

\subsection{Proof for \cref{thm:codet_error_converge}}
% \begin{customcorollary}{4.3}
%     If $\theta_x$ is large enough such that $\theta' n_{\hat y} < \theta_x n_y$, then the error probability $P(n_{\hat x}  n_{\hat y} > n_x n_y)$ can exponentially converge to 0 when $N\rightarrow\infty$. Otherwise, if $\theta_x$ is low enough such that $\theta' n_{\hat y} > \theta_x n_y$, the error probability converge to 1 when $N\rightarrow\infty$.
% \end{customcorollary}
\begin{proof}
    This proof is similar to that of \cref{thm:maxpass_ny}. Based on \cref{thm:codet}, denoting $P(n_{\hat x}  n_{\hat y} > n_x n_y)\sim \Phi(t)$ where $t=\mathcal{O}(\sqrt{N})$. If $\theta' n_{\hat y} < \theta_x n_y$, with the increase of $N$ we have $t<0$. According to \cref{thm:tail}:
    \begin{align*}
        P(n_{\hat x}  n_{\hat y} > n_x n_y)\sim \mathcal{O}\left(
            \nicefrac{
                c^{-\mathcal{O}(\sqrt{N})^2}
            }{
                \mathcal{O}(\sqrt{N})^2
            }
        \right)
        =\mathcal{O}\left(
            \nicefrac{
                c_1^{-N}
            }{
                \sqrt{N}
            }
        \right),
    \end{align*}
    where $c_1>1$ is some constant and $N\rightarrow\infty$.
    Conversely, if $\theta' n_{\hat y} > \theta_x n_y$,  with the increase of $N$ we have $t>0$, therefore $P(n_{\hat x}  n_{\hat y} > n_x n_y)\sim1-\mathcal{O}\left(
            \nicefrac{
                c_1^{-N}
            }{
                \sqrt{N}
            }
        \right)$. 
    
\end{proof}

% \subsection{Error bound for \ours}

% We show that the error bound (\ie, 
